# Supplementary material for: The $(2 + \delta)$-dimensional theory of the electromechanics of lipid membranes: I. Electrostatics
Source: arXiv:2301.09610 ancillary file (2023-01-23)
Supplement: Supplementary file 1 [file thin_film_electrostatics_SM.pdf]

# Supplementary Material

## The $(2 + \delta)$ -dimensional theory of the electromechanics of lipid membranes:

### I. Electrostatics

Yannick A. D. Omar<sup>1,†</sup>, Zachary G. Lipel<sup>1,§</sup>, and Kranthi K. Mandadapu<sup>1,2,\*</sup>

<sup>1</sup> Department of Chemical & Biomolecular Engineering, University of California, Berkeley, CA 94720, USA

<sup>2</sup> Chemical Sciences Division, Lawrence Berkeley National Laboratory, CA 94720, USA

## Contents

|          |                                                                   |           |
|----------|-------------------------------------------------------------------|-----------|
| <b>1</b> | <b>Maxwell's Equations</b>                                        | <b>1</b>  |
| <b>2</b> | <b>Derivation of an Effective Surface Equation for Gauss' Law</b> | <b>4</b>  |
| 2.1      | Governing Equations . . . . .                                     | 4         |
| 2.2      | Differential Geometry Preliminaries . . . . .                     | 5         |
| 2.3      | Dimension Reduction . . . . .                                     | 9         |
| <b>3</b> | <b>Derivation of Analytical Solutions</b>                         | <b>13</b> |
| 3.1      | Flat Geometry . . . . .                                           | 13        |
| 3.2      | Cylinders . . . . .                                               | 15        |
| 3.3      | Spheres . . . . .                                                 | 18        |
|          | <b>Supporting References</b>                                      | <b>20</b> |

## 1 Maxwell's Equations

We briefly revisit the fundamental equations governing the field of electrodynamics; a comprehensive treatment of the electrodynamics of continuous media can be found in Ref. [1]. Let  $\check{\mathbf{e}}$  and  $\mathbf{b}$  denote the electric and magnetic field and let  $\mathbf{d}$  and  $\mathbf{h}$  denote the charge and current potential. Furthermore, let  $q$  and  $\mathbf{j}$  be the total charge density and current density. The quantities  $\sigma$  and  $\mathbf{k}$  are the corresponding counterparts on a surface of discontinuity, namely the surface charge density and current. In a domain  $\mathcal{B} \subseteq \mathbb{R}^3$ , Maxwell's equations can be written as

$$\operatorname{div}(\mathbf{d}) = q, \quad \forall \check{\mathbf{x}} \in \mathcal{B}, \quad (1)$$

$$\operatorname{curl}(\mathbf{h}) - \mathbf{d}_{,t} = \mathbf{j}, \quad \forall \check{\mathbf{x}} \in \mathcal{B}, \quad (2)$$

$$\operatorname{div}(\mathbf{b}) = 0, \quad \forall \check{\mathbf{x}} \in \mathcal{B}, \quad (3)$$

$$\operatorname{curl}(\check{\mathbf{e}}) + \mathbf{b}_{,t} = \mathbf{0}, \quad \forall \check{\mathbf{x}} \in \mathcal{B}. \quad (4)$$

As in the main text, the *check* symbol is used to distinguish the electric field and positions from their corresponding counterparts in the dimensionally-reduced theory, as they are the only quantities

---

<sup>†</sup>yannick.omar@berkeley.edu

<sup>§</sup>zlipel@berkeley.edu

<sup>\*</sup>kranthi@berkeley.edu

that appear in both theories. On a surface of discontinuity  $\mathcal{S}$  with normal  $\bar{\mathbf{n}}$ , moving at velocity  $\bar{\mathbf{v}}$ , Maxwell's equations give rise to the jump conditions

$$\bar{\mathbf{n}} \cdot \llbracket \mathbf{d} \rrbracket = \sigma, \quad \forall \check{\mathbf{x}} \in \mathcal{S}, \quad (5)$$

$$\bar{\mathbf{n}} \times \llbracket \mathbf{h} \rrbracket + \bar{\mathbf{v}} \cdot \bar{\mathbf{n}} \llbracket \mathbf{d} \rrbracket = \mathbf{k}, \quad \forall \check{\mathbf{x}} \in \mathcal{S}, \quad (6)$$

$$\bar{\mathbf{n}} \cdot \llbracket \mathbf{b} \rrbracket = 0, \quad \forall \check{\mathbf{x}} \in \mathcal{S}, \quad (7)$$

$$\bar{\mathbf{n}} \times \llbracket \check{\mathbf{e}} \rrbracket + \bar{\mathbf{v}} \cdot \bar{\mathbf{n}} \llbracket \mathbf{b} \rrbracket = \mathbf{0}, \quad \forall \check{\mathbf{x}} \in \mathcal{S}. \quad (8)$$

Here,  $\llbracket \bullet \rrbracket = (\bullet)^+ - (\bullet)^-$  denotes the jump across the surface of discontinuity, where  $(\bullet)^\pm$  indicates evaluation in the bulk domain above and below the surface of discontinuity. The superscript “+” refers to the side to which  $\bar{\mathbf{n}}$  points, and “−” refers to the opposing side. A more detailed discussion about jump conditions at surfaces of discontinuities can be found in Ref. [2].

Equations (1)–(8) are not well-posed—there are more unknowns than equations. Thus, we assume there exists an aether frame in which the so-called aether relations hold,

$$\mathbf{d} = \varepsilon_0 \check{\mathbf{e}}, \quad (9)$$

$$\mathbf{h} = \frac{1}{\mu_0} \mathbf{b}, \quad (10)$$

where  $\varepsilon_0$  and  $\mu_0$  denote universal constants, often referred to as permittivity and permeability of free space. As discussed by Kovetz [1], these relations hold true in any aether frame and are independent of the material occupying the point under consideration. With the aether relations, Eqs. (9) and (10), Eqs. (1)–(8) become well-posed. We emphasize here that the charge densities  $q$  and  $\sigma$  as well as the charge current densities  $\mathbf{j}$  and  $\mathbf{k}$  refer to the *total* charge and current densities.

To account for a material specific response to external fields, we split the charge and current densities into free and bound contributions:

$$q = q_f + q_b, \quad (11)$$

$$\sigma = \sigma_f + \sigma_b, \quad (12)$$

$$\mathbf{j} = \mathbf{j}_f + \mathbf{j}_b, \quad (13)$$

$$\mathbf{k} = \mathbf{k}_f + \mathbf{k}_b, \quad (14)$$

where the subscripts “f” and “b” denote free and bound quantities, respectively. Correspondingly, we split the charge and current potentials into free and bound contributions:

$$\mathbf{d} = \mathbf{d}_f - \mathbf{p}, \quad (15)$$

$$\mathbf{h} = \mathbf{h}_f + \mathbf{m}, \quad (16)$$

where  $\mathbf{p}$  and  $\mathbf{m}$  denote the polarization and magnetization field, respectively, and the negative sign in front of  $\mathbf{p}$  is purely conventional. Equations (1) and (2) can be derived from charge conservation such that they hold for both the free and bound fields separately. Therefore, equivalently to Eqs. (1), (2), (5), and (6), we find

$$\text{div}(\mathbf{d}_f) = q_f, \quad \forall \check{\mathbf{x}} \in \mathcal{B}, \quad (17)$$

$$\text{curl}(\mathbf{h}_f) - \mathbf{d}_{f,t} = \mathbf{j}_f, \quad \forall \check{\mathbf{x}} \in \mathcal{B}, \quad (18)$$

$$\bar{\mathbf{n}} \cdot \llbracket \mathbf{d}_f \rrbracket = \sigma \quad , \quad \forall \tilde{\mathbf{x}} \in \mathcal{S} \quad , \quad (19)$$

$$\bar{\mathbf{n}} \times \llbracket \mathbf{h}_f \rrbracket + \bar{\mathbf{v}} \cdot \bar{\mathbf{n}} \llbracket \mathbf{d}_f \rrbracket = \mathbf{k}_f \quad , \quad \forall \tilde{\mathbf{x}} \in \mathcal{S} \quad . \quad (20)$$

The remaining Maxwell's equations are unaffected by the split into free and bound fields. However, we note that the aether relations, Eqs. (9) and (10), do not apply to the free fields. Therefore, the problem is currently not well-posed and requires additional constitutive relations.

Before introducing constitutive relations for the polarization and magnetization fields, we specialize Eqs. (3), (4), (7), (8) and (17)–(20) to the case of electrostatics. The electrostatic equations can be derived by assuming that  $\mathbf{d}_{f,t}$ ,  $\mathbf{b}_{f,t}$ ,  $\mathbf{j}_f$ ,  $\bar{\mathbf{v}}$ , and  $\mathbf{k}_f$  vanish identically everywhere [1]. In order to decouple Eqs. (17)–(20) from Eqs. (3), (4), (7), and (8), we assume that the charge densities  $q_f$  and  $\sigma_f$ , and polarization  $\mathbf{p}$  are independent of the magnetic field  $\mathbf{b}$ . According to the framework of linear irreversible thermodynamics, the latter condition implies that the magnetization  $\mathbf{m}$  has to vanish [3], yielding the electrostatic equations

$$\text{div}(\mathbf{d}_f) = q \quad , \quad \forall \tilde{\mathbf{x}} \in \mathcal{B} \quad , \quad (21)$$

$$\text{curl}(\check{\mathbf{e}}) = \mathbf{0} \quad , \quad \forall \tilde{\mathbf{x}} \in \mathcal{B} \quad , \quad (22)$$

$$\bar{\mathbf{n}} \cdot \llbracket \mathbf{d}_f \rrbracket = \sigma \quad , \quad \forall \tilde{\mathbf{x}} \in \mathcal{S} \quad , \quad (23)$$

$$\bar{\mathbf{n}} \times \llbracket \check{\mathbf{e}} \rrbracket = \mathbf{0} \quad , \quad \forall \tilde{\mathbf{x}} \in \mathcal{S} \quad . \quad (24)$$

The approach described in the above paragraph to derive the electrostatic equations is restrictive. However, the electrostatic equations are also valid under an appropriate separation of time scales [4]. Let  $\ell$  denote a characteristic length scale and  $\tau$  a characteristic dynamical time scale associated with a phenomena that one wishes to study. Non-dimensionalization of Maxwell's equations shows that  $\tau_e = \varepsilon_0/\sigma_c$  is the characteristic charge relaxation time scale, where  $\sigma_c$  is the conductivity, and  $\tau_m = \mu_0\sigma_c\ell^2$  is the magnetic diffusion time scale [4]. If  $\ell^2/c^2 \ll \tau^2$ , where  $c$  is the speed of light, and  $\tau_e > \tau_m$ , Maxwell's equations decouple and simplify to the electrostatic equations Eqs. (21)–(24) as discussed in detail in Ref. [4].

To close Eqs. (21)–(24), we introduce the constitutive relation of a linear dielectric [3],

$$\mathbf{p} = (\varepsilon - \varepsilon_0) \check{\mathbf{e}} \quad . \quad (25)$$

Using Eq. (15), we then find

$$\mathbf{d}_f = \varepsilon \check{\mathbf{e}} \quad . \quad (26)$$

Therefore, the electrostatic equations, Eqs. (21)–(24), become

$$\text{div}(\varepsilon \check{\mathbf{e}}) = q_f \quad , \quad \forall \tilde{\mathbf{x}} \in \mathcal{B} \quad , \quad (27)$$

$$\text{curl}(\check{\mathbf{e}}) = \mathbf{0} \quad , \quad \forall \tilde{\mathbf{x}} \in \mathcal{B} \quad , \quad (28)$$

$$\bar{\mathbf{n}} \cdot \llbracket \varepsilon \check{\mathbf{e}} \rrbracket = \sigma_f \quad , \quad \forall \tilde{\mathbf{x}} \in \mathcal{S} \quad , \quad (29)$$

$$\bar{\mathbf{n}} \times \llbracket \check{\mathbf{e}} \rrbracket = \mathbf{0} \quad , \quad \forall \tilde{\mathbf{x}} \in \mathcal{S} \quad . \quad (30)$$

Both in the bulk domain  $\mathcal{B}$  and on the surface of discontinuity  $\mathcal{S}$ , Eqs. (27)–(30) yield four equations for three unknowns. According to the Helmholtz decomposition however, every sufficiently smooth vector field can be decomposed into a curl-free field and a divergence-free field,

$$\check{\mathbf{e}} = -\text{grad}(\check{\phi}) + \text{curl}(\mathbf{A}) \quad , \quad (31)$$

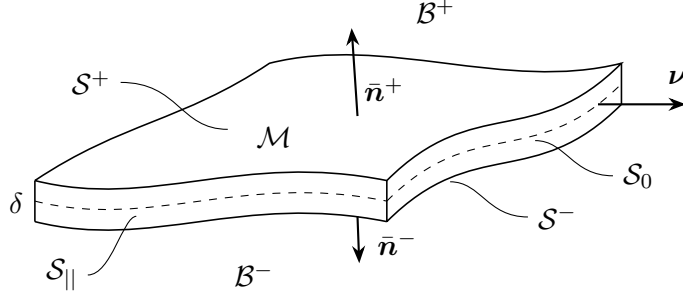

Figure 1: Schematic of the setup used for our derivation. We consider a shell-like body  $\mathcal{M}$  with thickness  $\delta$  that separates the two bulk domains  $\mathcal{B}^+$  and  $\mathcal{B}^-$ .

where  $\check{\phi}$  and  $\mathbf{A}$  are some scalar and vector fields, respectively. Furthermore, according to Eq. (27) and (28), we can set, without loss of generality,  $\mathbf{A} = 0$ , such that we are left with

$$-\varepsilon \Delta \check{\phi} = q_f, \quad \forall \check{\mathbf{x}} \in \mathcal{B}, \quad (32)$$

$$-\bar{\mathbf{n}} \cdot \llbracket \varepsilon \text{grad}(\check{\phi}) \rrbracket = \sigma_f, \quad \forall \check{\mathbf{x}} \in \mathcal{S}, \quad (33)$$

$$\llbracket \check{\phi} \rrbracket = 0, \quad \forall \check{\mathbf{x}} \in \mathcal{S}, \quad (34)$$

where we now identify  $\check{\phi}$  as the electric potential. Equation (34) is not derived here but follows from the integral form of Coulomb's law for continuous charges [5]. Furthermore, we assume that the permittivity is constant in the bulk domain  $\mathcal{B}$  and omit the condition following from Eq. (30) as it is trivially satisfied due to Eq. (34). Equations (32)–(34) serve as the starting point for the derivation of the  $(2 + \delta)$ -dimensional theory, where we will omit the subscript f for free quantities for brevity.

## 2 Derivation of an Effective Surface Equation for Gauss' Law

In this section, a detailed derivation of the  $(2 + \delta)$ -dimensional theory for the electrostatics of thin films is provided. We begin by revisiting the three-dimensional theory governing the electrostatics of thin films and subsequently apply the dimension reduction procedure introduced in Sec. 3.2 of the main text.

### 2.1 Governing Equations

The equations governing the electrostatics of a thin film, schematically shown in Fig. 1, are given by

$$\Delta \check{\phi}_{\mathcal{B}^-} = -q_{\mathcal{B}^-} / \varepsilon_{\mathcal{B}^-}, \quad \forall \check{\mathbf{x}} \in \mathcal{B}^-, \quad (35)$$

$$\llbracket \check{\phi} \rrbracket = 0, \quad \forall \check{\mathbf{x}} \in \mathcal{S}^-, \quad (36)$$

$$\bar{\mathbf{n}}^+ \cdot \llbracket \varepsilon \check{\mathbf{e}} \rrbracket = \sigma^-, \quad \forall \check{\mathbf{x}} \in \mathcal{S}^-, \quad (37)$$

$$\varepsilon_{\mathcal{M}} \Delta \check{\phi}_{\mathcal{M}} = 0, \quad \forall \check{\mathbf{x}} \in \mathcal{M}, \quad (38)$$

$$\bar{\mathbf{n}}^- \cdot \llbracket \varepsilon \check{\mathbf{e}} \rrbracket = \sigma^+, \quad \forall \check{\mathbf{x}} \in \mathcal{S}^+, \quad (39)$$

$$[[\check{\phi}]] = 0 \quad , \quad \forall \check{\mathbf{x}} \in \mathcal{S}^+ , \quad (40)$$

$$\Delta \check{\phi}_{B^+} = -q_{B^+}/\varepsilon_{B^+} , \quad \forall \check{\mathbf{x}} \in \mathcal{B}^+ . \quad (41)$$

The superscripts  $\pm$  indicate quantities above and below the membrane (Fig. 1), the subscripts  $B^\pm$  and  $M$  indicate the two bulk domains and membrane, respectively,  $\bar{\mathbf{n}}^\pm$  denotes the normal to  $\mathcal{S}^\pm$ , and all other symbols carry the same meaning as in Sec. 1. The *check* symbol is used on some quantities to distinguish them from their counterparts in the dimensionally-reduced theory.

Equations (35)–(41) are closed with the boundary conditions on the lateral surface  $\mathcal{S}_{||}$  with outward-pointing normal  $\boldsymbol{\nu}$ ,

$$\check{\phi}_M = \bar{\phi}_M , \quad \forall \check{\mathbf{x}} \in \mathcal{S}_{||D} , \quad (42)$$

$$-\boldsymbol{\nu} \cdot \text{grad}(\check{\phi}_M) = \bar{e} \quad , \quad \forall \check{\mathbf{x}} \in \mathcal{S}_{||N} , \quad (43)$$

where  $\bar{\phi}_M$  and  $\bar{e}$  are the prescribed potential and electric field, respectively, and  $\mathcal{S}_{||} = \mathcal{S}_{||D} \cup \mathcal{S}_{||N}$  and  $\mathcal{S}_{||D} \cap \mathcal{S}_{||N} = \emptyset$ . The remaining boundary conditions for  $\check{\phi}_{B^\pm}$  are of no consequence for the derivation of the dimensionally-reduced theory and are thus omitted here.

## 2.2 Differential Geometry Preliminaries

In the following derivations, vectors and tensors are denoted by bold letters and matrices are denoted using square brackets. Subscripts and superscripts indicate covariant and contravariant components, respectively, and repeated sub- and superscripts imply Einstein's summation convention. The tensors considered in this article are symmetric such that the order of co- and contravariant components is inconsequential and is therefore not explicitly indicated. Greek indices take values  $\{1, 2\}$  while Latin indices take values  $\{1, 2, 3\}$ . For some function  $f$ , the short-hand notation  $f(\zeta^\alpha)$  implies  $f(\zeta^1, \zeta^2)$  and an analogous short-hand notation is used with Latin indices. Partial derivatives are denoted by a comma, covariant derivatives of a vector are denoted by a vertical bar, and *surface* covariant derivatives of vectors and tensors are denoted by colons and semicolons, respectively.

We begin by recalling that the assumption of Kirchhoff-Love kinematics implies the position vector  $\mathbf{x}$  can be expressed as

$$\mathbf{x} = \mathbf{x}_0 P_0(\theta(\zeta^3)) + \frac{\delta}{2} \mathbf{n} P_1(\theta(\zeta^3)) , \quad (44)$$

where  $\mathbf{x}_0$  denotes a point on the mid-surface,  $\mathbf{n}$  is the normal to the mid-surface,  $P_i(\theta(\zeta^3))$  is the  $i^{\text{th}}$  Chebyshev polynomial, and  $\theta : \Xi \rightarrow (-1, 1)$  maps from the parametric domain  $\Xi$  onto the domain of the Chebyshev polynomials. Furthermore, recall that the coefficients  $\mathbf{x}_0$  and  $\mathbf{n}$  depend on the mid-plane parametrization  $\zeta^\alpha$ . In the following, we omit, where convenient, the 0<sup>th</sup> order Chebyshev polynomial,  $P_0(\theta) = 1$ , and the explicit dependence of  $\theta$  on  $\zeta^3$ .

Using Eq. (44), we can now define the in-plane, covariant basis vectors as

$$\mathbf{g}_\alpha := \frac{\partial \mathbf{x}}{\partial \zeta^\alpha} \quad (45)$$

$$= \mathbf{a}_\alpha + \frac{\delta}{2} \mathbf{n}_{,\alpha} P_1(\theta) \quad (46)$$

$$= \mathbf{a}_\alpha - \frac{\delta}{2} b_\alpha^\beta \mathbf{a}_\beta P_1(\theta) , \quad (47)$$

where we defined  $\mathbf{a}_\alpha := \partial \mathbf{x}_0 / \partial \zeta^\alpha$  and used the Weingarten formula with the curvature tensor components  $b_{\alpha\gamma} = \mathbf{a}_{\alpha,\gamma} \cdot \mathbf{n}$  and the contravariant metric tensor  $a^{\gamma\beta}$ , such that  $b_\alpha^\beta = b_{\alpha\gamma} a^{\gamma\beta}$ . The third basis vector is calculated to be

$$\mathbf{g}_3 := \frac{\partial \mathbf{x}}{\partial \zeta^3} = \mathbf{n} , \quad (48)$$

implying that  $\bar{\mathbf{n}}^+ = \bar{\mathbf{n}}^- = \mathbf{n}$ . Restricting the basis vectors in Eqs. (47) and (48) to the mid-surface yields

$$\mathbf{g}_\alpha|_{\zeta^3=0} = \mathbf{a}_\alpha , \quad (49)$$

$$\mathbf{g}_3|_{\zeta^3=0} = \mathbf{n} . \quad (50)$$

Therefore, we identify  $\{\mathbf{a}_\alpha, \mathbf{n}\}$  as the basis on the mid-surface, satisfying  $\mathbf{a}_\alpha \cdot \mathbf{n} = 0$ .

In curvilinear coordinates, the Laplacian of the potential  $\check{\phi}$  can be written as [6]

$$\Delta \check{\phi} = \check{\phi}_{,i}|_j g^{ij} \quad (51)$$

$$= \left( \check{\phi}_{,ij} - \Gamma_{ij}^k \check{\phi}_{,k} \right) g^{ij} , \quad (52)$$

where  $\check{\phi}_{,i} = \partial \check{\phi} / \partial \zeta^i$ ,  $\check{\phi}_{,i}|_j$  is the covariant derivative of  $\phi_{,i}$ ,  $g^{ij} = \mathbf{g}^i \cdot \mathbf{g}^j$  is the contravariant metric, and  $\Gamma_{ij}^k$  is the Christoffel symbol of the second kind, defined as

$$\Gamma_{ij}^k = \mathbf{g}_{i,j} \cdot \mathbf{g}^k . \quad (53)$$

Here,  $\mathbf{g}^k$  denotes the contravariant basis vector, related to the covariant basis vectors by

$$\mathbf{g}^k = g^{kl} \mathbf{g}_l . \quad (54)$$

From  $[g^{ij}] = [g_{ij}]^{-1}$  and Eq. (47), it becomes apparent that  $g^{ij}$ ,  $\mathbf{g}^k$ , and  $\Gamma_{ij}^k$  are rational polynomials. This complicates evaluation of the inner products required in the proposed dimension reduction method. Therefore, we find approximate, non-rational polynomial expressions for these quantities, requiring the truncation of small terms using the geometric properties of the thin film. To that end, we introduce the principal curvatures of a surface, denoted by  $\kappa_\alpha$ . Furthermore, we define the mean and Gaussian curvatures as the trace and determinant of the curvature tensor  $\mathbf{b}$ :

$$H = \frac{1}{2} \text{tr } \mathbf{b} , \quad (55)$$

$$K = \det \mathbf{b} , \quad (56)$$

where  $\text{tr}$  and  $\det$  denote the trace and determinant, respectively. The mean and Gaussian curvatures are related to the principal curvatures by

$$H = \frac{1}{2} (\kappa_1 + \kappa_2) , \quad (57)$$

$$K = \kappa_1 \kappa_2 . \quad (58)$$

We now make the assumption that the principal curvatures are small compared to the thickness of the thin film, i.e.

$$(\delta \kappa_\alpha)^2 \ll 1 , \quad (59)$$

as is often found for lipid membranes. While Eq. (59) also implies

$$(\delta H)^2 \ll 1 , \quad (60)$$

$$\delta^2 |K| \ll 1 , \quad (61)$$

the former two inequalities do not imply Eq. (59). However, Eq. (59) allows us to further simplify our derivations in the following.

In particular, we need to estimate the order of magnitude of the curvature tensor  $\mathbf{b}$ . Denoting the orthonormal eigenvectors of  $\mathbf{b}$  by  $\mathbf{l}_\alpha = \mathbf{l}^\alpha$ , the spectral decomposition of the curvature tensor becomes

$$\mathbf{b} = \sum_{\alpha=1}^2 \kappa_\alpha \mathbf{l}_\alpha \otimes \mathbf{l}_\alpha . \quad (62)$$

Using Eq. (62), we can estimate the order of magnitude of  $\mathbf{b}$  acting on an arbitrary symmetric tensor  $\mathbf{A} = A_\alpha^\beta \mathbf{l}^\alpha \otimes \mathbf{l}_\beta$ . Taking the inner product of  $\mathbf{A}$  and  $\mathbf{b}$ , we find

$$(\delta \mathbf{b})^2 : \mathbf{A} = \sum_{\alpha=1}^2 (\delta \kappa_\alpha)^2 A_\alpha^\alpha , \quad (63)$$

where the colon indicates a double contraction. Similarly, we find

$$\mathbf{I}_0 : \mathbf{A} = A_\alpha^\alpha , \quad (64)$$

where  $\mathbf{I}_0 = \mathbf{a}_\alpha \otimes \mathbf{a}^\alpha = \mathbf{l}_\alpha \otimes \mathbf{l}^\alpha$  is the unit tensor on the tangent plane to  $\mathcal{S}_0$ . The quantities in Eqs. (63) and (64) are invariant, implying

$$(\delta \mathbf{b})^2 : \mathbf{A} \ll \mathbf{I}_0 : \mathbf{A} . \quad (65)$$

Next, we derive an order of magnitude estimate for the components of the curvature tensor. The Cayley-Hamilton theorem applied to the curvature tensor reads [6]

$$\mathbf{b}^2 - 2H\mathbf{b} + K\mathbf{I}_0 = \mathbf{0} . \quad (66)$$

Multiplying Eq. (66) through by  $\delta^3 \mathbf{b}$  and substituting Eq. (66) back, we find

$$\delta^3 \mathbf{b}^3 - \delta^3 (4H^2 - K) \mathbf{b} + 2\delta^3 H K \mathbf{I}_0 = \mathbf{0} . \quad (67)$$

With Eqs. (60) and (61), Eq. (67) is an estimate of the order of magnitude of the cube of the curvature tensor when compared to  $\mathbf{b}$  and  $\mathbf{I}$ . In the remainder of the derivation, we often discard small terms using Eqs. (60), (61), (65), and (67). For notational simplicity, the omitted terms are replaced by  $\mathcal{O}((\delta \kappa)^n)$  for some integer  $n$  and  $\kappa = \max_\alpha (|\kappa_\alpha|)$  to indicate the order of truncation.

We are now equipped to find an approximate polynomial expression for  $\mathbf{g}^k$ . Equations (47) and (48) yield

$$g_{ij} = \begin{bmatrix} [g_{\alpha\beta}] & \mathbf{0} \\ \mathbf{0} & 1 \end{bmatrix} , \quad (68)$$

and consequently

$$g^{ij} = \begin{bmatrix} [g_{\alpha\beta}]^{-1} & \mathbf{0} \\ \mathbf{0} & 1 \end{bmatrix}, \quad (69)$$

such that we only have to concern ourselves with finding an expression for the in-plane metric  $g_{\alpha\beta}$  and its inverse. For notational convenience, the following derivation is expressed in standard polynomial form rather than Chebyshev polynomials. From Eq. (47), we then obtain

$$g_{\alpha\beta} = a_{\alpha\beta} - \delta b_{\alpha\beta} \theta + \frac{\delta^2}{4} b_{\alpha}^{\gamma} b_{\gamma\beta} \theta^2. \quad (70)$$

Taking the determinant of the metric yields

$$\det(g_{\alpha\beta}) = \det(a_{\alpha\beta}) (1 - 2H\delta\theta) + \mathcal{O}((\delta\kappa)^2), \quad (71)$$

and Taylor-expanding the inverse of the determinant of the metric yields

$$\frac{1}{\det(g_{\alpha\beta})} = \frac{1}{\det(a_{\alpha\beta})} (1 + 2H\delta\theta) + \mathcal{O}((\delta\kappa)^2). \quad (72)$$

Using  $[g_{\alpha\beta}]^{-1} = [g^{\alpha\beta}]$ , Cramer's rule, and Eq. (72), the contravariant metric becomes

$$g^{\alpha\beta} = \frac{1}{\det(a_{\alpha\beta})} \varepsilon^{\alpha\gamma} g_{\delta\gamma} \varepsilon^{\beta\delta} \left( 1 + 2H\delta\theta + \mathcal{O}((\delta\kappa)^2) \right), \quad (73)$$

where  $\varepsilon^{\alpha\beta}$  is the unit alternator, defined as

$$\varepsilon^{\alpha\beta} = \begin{bmatrix} 0 & 1 \\ -1 & 0 \end{bmatrix}. \quad (74)$$

Simplifying Eq. (73) further yields

$$g^{\alpha\beta} = a^{\alpha\beta} + \delta b^{\alpha\beta} \theta + \frac{3\delta^2}{2} H b^{\alpha\beta} \theta^2 + \mathcal{O}((\delta\kappa)^2) \quad (75)$$

where the Cayley-Hamilton theorem was used [7].

We obtain an expression for the contravariant basis vectors by substituting Eq. (75) into Eq. (54) and using Eq. (66), yielding

$$\mathbf{g}^{\alpha} = \mathbf{a}^{\alpha} + \frac{\delta}{2} b_{\beta}^{\alpha} \mathbf{a}^{\beta} + \frac{\delta^2}{2} H b_{\beta}^{\alpha} \mathbf{a}^{\beta} + \mathcal{O}((\delta\kappa)^2) \quad (76)$$

$$= \left( \delta_{\beta}^{\alpha} + \frac{\delta^2}{4} H b_{\beta}^{\alpha} \right) \mathbf{a}^{\beta} P_0(\theta) + \frac{\delta}{2} b_{\beta}^{\alpha} \mathbf{a}^{\beta} P_1(\theta) + \frac{\delta^2}{4} H b_{\beta}^{\alpha} \mathbf{a}^{\beta} P_2(\theta) + \mathcal{O}((\delta\kappa)^2), \quad (77)$$

Furthermore, from Eq. (69), it immediately follows that

$$\mathbf{g}^3 = \mathbf{g}_3 = \mathbf{n}. \quad (78)$$

Given approximate expressions for  $g^{ij}$  and  $\mathbf{g}^k$ , we are left with finding approximate expressions for the Christoffel symbols  $\Gamma_{ij}^k$ . With Eqs. (46), (76) and (78), the dot product in Eq. (53) can

be evaluated. However, considering the structure of  $g^{\alpha\beta}$ , we only require the following Christoffel symbols to evaluate Eq. (52):

$$\Gamma_{\alpha\beta}^\gamma = {}^0\Gamma_{\alpha\beta}^\gamma - \frac{\delta}{2}b_{\alpha;\beta}^\gamma\theta - \frac{\delta^2}{4}b_{\alpha;\beta}^\mu b_\mu^\gamma\theta^2 - \frac{\delta^3}{4}Hb_{\alpha;\beta}^\mu b_\mu^\gamma\theta^3 + \mathcal{O}\left((\delta\kappa)^2\right), \quad (79)$$

$$\Gamma_{\alpha\beta}^3 = b_{\alpha\beta} - \frac{\delta}{2}b_\alpha^\gamma b_{\gamma\beta}\theta, \quad (80)$$

$$\Gamma_{33}^\gamma = 0, \quad (81)$$

$$\Gamma_{33}^3 = \Gamma_{3\alpha}^3 = 0. \quad (82)$$

In Eq. (79),  ${}^0\Gamma_{\alpha\beta}^\gamma := \mathbf{a}_{\alpha,\beta} \cdot \mathbf{a}^\gamma$  denotes the Christoffel symbol on the mid-surface and a semicolon indicates the surface covariant derivative of a tensor. Moreover, to obtain Eqs. (79) and (80), we used Eq. (67), the relations

$$\mathbf{n}_{,3} = \mathbf{0}, \quad (83)$$

$$\mathbf{n}_{,\alpha} \cdot \mathbf{n} = 0, \quad (84)$$

as well as

$$\mathbf{n}_{,\alpha\beta} = -\left(b_{\alpha}^\delta \mathbf{a}_\delta\right)_{,\beta} \quad (85)$$

$$= -\left(b_{\alpha,\beta}^\delta \mathbf{a}_\delta + b_\alpha^\delta {}^0\Gamma_{\delta\beta}^\epsilon \mathbf{a}_\epsilon + b_\alpha^\delta b_{\delta\beta} \mathbf{n}\right), \quad (86)$$

implying

$$\mathbf{n}_{,\alpha\beta} \cdot \mathbf{a}^\gamma + {}^0\Gamma_{\alpha\beta}^\delta b_\delta^\gamma = -b_{\alpha;\beta}^\gamma. \quad (87)$$

### 2.3 Dimension Reduction

We now apply the dimension reduction procedure introduced in Sec. 3.2 of the main text to find the dimensionally-reduced equation corresponding to Eq. (38). This requires evaluating Eq. (52) using the expressions for the inverse metric and Christoffel symbols derived in Sec. 2.2 as well as the expansion of the potential introduced in Sec. 4 of the main text:

$$\phi = \phi_0 P_0(\theta) + \phi_1 P_1(\theta) + \phi_2 P_2(\theta). \quad (88)$$

The partial derivatives appearing in Eq. (52) evaluate to

$$\phi_{,\alpha\beta} = \phi_{0,\alpha\beta} P_0(\theta) + \phi_{1,\alpha\beta} P_1(\theta) + \phi_{2,\alpha\beta} P_2(\theta) \quad (89)$$

$$\phi_{,33} = \frac{16}{\delta^2} \phi_2, \quad (90)$$

and multiplication by the metric tensor yields

$$g^{\alpha\beta} \phi_{,\alpha\beta} \stackrel{0}{=} \phi_{0,\alpha\beta} \left( a^{\alpha\beta} + \frac{3\delta^2}{4} H b^{\alpha\beta} \right) + \frac{\delta}{2} b^{\alpha\beta} \phi_{1,\alpha\beta} + \frac{3\delta^2}{16} b^{\alpha\gamma} b_\gamma^\beta \phi_{2,\alpha\beta} + \mathcal{O}\left((\delta\kappa)^2\right), \quad (91)$$

$$g^{33} \phi_{,33} = \frac{16}{\delta^2} \phi_2, \quad (92)$$

where  $\stackrel{k}{=}$  indicates that the expression following the equal sign is truncated after the  $k^{\text{th}}$  Chebyshev polynomial. In Eq. (91), the term highlighted in orange is negligible based on Eqs. (65) and (66).

Next, the Christoffel symbol terms in Eq. (52) are expanded as

$$\begin{aligned} \phi_{,\gamma} \Gamma_{\alpha\beta}^{\gamma} = & (\phi_{0,\gamma} P_0(\theta) + \phi_{1,\gamma} P_1(\theta) + \phi_{2,\gamma} P_2(\theta)) \times \\ & \left( \left( {}^0\Gamma_{\alpha\beta}^{\gamma} - \frac{\delta^2}{8} b_{\alpha;\beta}^{\mu} b_{\mu}^{\gamma} \right) P_0(\theta) - \left( \frac{\delta}{2} b_{\alpha;\beta}^{\gamma} + \frac{3\delta^3}{16} H b_{\alpha;\beta}^{\mu} b_{\mu}^{\gamma} \right) P_1(\theta) \right. \\ & \left. - \frac{\delta^2}{8} b_{\alpha;\beta}^{\mu} b_{\mu}^{\gamma} P_2(\theta) - \frac{\delta^3}{16} H b_{\alpha;\beta}^{\mu} b_{\mu}^{\gamma} P_3(\theta) + \mathcal{O}((\delta\kappa)^2) \right) \end{aligned} \quad (93)$$

$$\begin{aligned} \stackrel{2}{=} & P_0(\theta) \left\{ \phi_{0,\gamma} \left( {}^0\Gamma_{\alpha\beta}^{\gamma} - \frac{\delta^2}{8} b_{\alpha;\beta}^{\mu} b_{\mu}^{\gamma} \right) - \phi_{1,\gamma} \frac{\delta}{4} \left( b_{\alpha;\beta}^{\gamma} + \frac{3\delta^2}{8} H b_{\alpha;\beta}^{\mu} b_{\mu}^{\gamma} \right) - \phi_{2,\gamma} \frac{\delta^2}{16} b_{\alpha;\beta}^{\mu} b_{\mu}^{\gamma} \right\} \\ & P_1(\theta) \left\{ -\phi_{0,\gamma} \frac{\delta}{2} \left( b_{\alpha;\beta}^{\gamma} + \frac{3\delta^2}{8} H b_{\alpha;\beta}^{\mu} b_{\mu}^{\gamma} \right) + \phi_{1,\gamma} \left( {}^0\Gamma_{\alpha\beta}^{\gamma} - \frac{3\delta^2}{16} b_{\alpha;\beta}^{\mu} b_{\mu}^{\gamma} \right) \right. \\ & \quad \left. - \phi_{2,\gamma} \frac{\delta}{4} \left( b_{\alpha;\beta}^{\gamma} + \frac{\delta^2}{2} H b_{\alpha;\beta}^{\mu} b_{\mu}^{\gamma} \right) \right\} \\ & P_2(\theta) \left\{ -\phi_{0,\gamma} \frac{\delta^2}{8} b_{\alpha;\beta}^{\mu} b_{\mu}^{\gamma} - \phi_{1,\gamma} \frac{\delta}{4} \left( b_{\alpha;\beta}^{\gamma} + \frac{\delta^2}{2} H b_{\alpha;\beta}^{\mu} b_{\mu}^{\gamma} \right) + \phi_{2,\gamma} \left( {}^0\Gamma_{\alpha\beta}^{\gamma} - \frac{\delta^2}{8} b_{\alpha;\beta}^{\mu} b_{\mu}^{\gamma} \right) \right\} \\ & + \mathcal{O}((\delta\kappa)^2), \end{aligned} \quad (94)$$

and

$$\begin{aligned} \phi_{,3} \Gamma_{\alpha\beta}^3 = & \left( \frac{2}{\delta} \phi_1 P_0(\theta) + \frac{8}{\delta} \phi_2 P_1(\theta) \right) \times \\ & \left( b_{\alpha\beta} P_0(\theta) - \frac{\delta}{2} (2H b_{\alpha\beta} - K a_{\alpha\beta}) P_1(\theta) \right) \end{aligned} \quad (95)$$

$$\begin{aligned} = & P_0(\theta) \left\{ \frac{2}{\delta} \phi_1 b_{\alpha\beta} - 2\phi_2 (2H b_{\alpha\beta} - K a_{\alpha\beta}) \right\} + \\ & P_1(\theta) \left\{ \phi_1 (2H b_{\alpha\beta} - K a_{\alpha\beta}) + \frac{8}{\delta} \phi_2 b_{\alpha\beta} \right\} + \\ & P_2(\theta) \left\{ -2\phi_2 (2H b_{\alpha\beta} - K a_{\alpha\beta}) \right\}. \end{aligned} \quad (96)$$

Contraction with the metric tensor then yields

$$\begin{aligned} g^{\alpha\beta} \phi_{,\gamma} \Gamma_{\alpha\beta}^{\gamma} \stackrel{0}{=} & \phi_{0,\gamma} \left\{ \left( {}^0\Gamma_{\alpha\beta}^{\gamma} - \frac{\delta^2}{8} b_{\alpha;\beta}^{\mu} b_{\mu}^{\gamma} \right) \left( a^{\alpha\beta} + \frac{3\delta^2}{4} H b^{\alpha\beta} \right) - \frac{\delta^2}{4} \left( b_{\alpha;\beta}^{\gamma} + \frac{9\delta^2}{16} H b_{\alpha;\beta}^{\mu} b_{\mu}^{\gamma} \right) b^{\alpha\beta} \right\} \\ & \phi_{1,\gamma} \left\{ -\frac{\delta}{4} \left( b_{\alpha;\beta}^{\gamma} + \frac{3\delta^2}{8} H b_{\alpha;\beta}^{\mu} b_{\mu}^{\gamma} \right) \left( a^{\alpha\beta} + \frac{3\delta^2}{4} H b^{\alpha\beta} \right) \right. \\ & \quad \left. + \frac{\delta}{2} b^{\alpha\beta} \left( {}^0\Gamma_{\alpha\beta}^{\gamma} - \frac{3\delta^2}{16} b_{\alpha;\beta}^{\mu} b_{\mu}^{\gamma} \right) - \frac{3\delta^3}{32} H b^{\alpha\beta} \left( b_{\alpha;\beta}^{\gamma} + \frac{\delta^2}{2} H b_{\alpha;\beta}^{\mu} b_{\mu}^{\gamma} \right) \right\} \\ & \phi_{2,\gamma} \left\{ -\frac{\delta^2}{16} b_{\alpha;\beta}^{\mu} b_{\mu}^{\gamma} \left( a^{\alpha\beta} + \frac{3\delta^2}{4} H b^{\alpha\beta} \right) \right\} \end{aligned}$$

$$- \frac{\delta^2}{8} b^{\alpha\beta} \left( b_{\alpha;\beta}^\gamma + \frac{\delta^2}{2} H b_{\alpha;\beta}^\mu b_\mu^\gamma \right) + \frac{3\delta^2}{8} H b^{\alpha\beta} \left( {}^0\Gamma_{\alpha\beta}^\gamma - \frac{\delta^2}{8} b_{\alpha;\beta}^\mu b_\mu^\gamma \right) \Big\} + \mathcal{O}\left((\delta\kappa)^2\right) \quad (97)$$

$$\begin{aligned} &= \phi_{0,\gamma} \left\{ \left( {}^0\Gamma_{\alpha\beta}^\gamma - \frac{\delta^2}{8} b_{\alpha;\beta}^\mu b_\mu^\gamma \right) a^{\alpha\beta} - \frac{\delta^2}{4} b_{\alpha;\beta}^\gamma b^{\alpha\beta} \right\} \\ &\quad \phi_{1,\gamma} \left\{ -\frac{\delta}{4} \left( b_{\alpha;\beta}^\gamma + \frac{3\delta^2}{8} H b_{\alpha;\beta}^\mu b_\mu^\gamma \right) a^{\alpha\beta} + \frac{\delta}{2} b^{\alpha\beta} \left( {}^0\Gamma_{\alpha\beta}^\gamma - \frac{3\delta^2}{16} b_{\alpha;\beta}^\mu b_\mu^\gamma \right) \right\} \\ &\quad \phi_{2,\gamma} \left\{ -\frac{\delta^2}{16} b_{\alpha;\beta}^\mu b_\mu^\gamma a^{\alpha\beta} - \frac{\delta^2}{8} b^{\alpha\beta} b_{\alpha;\beta}^\gamma + \frac{3\delta^2}{8} H {}^0\Gamma_{\alpha\beta}^\gamma b^{\alpha\beta} \right\} + \mathcal{O}\left((\delta\kappa)^2\right), \end{aligned} \quad (98)$$

and

$$\begin{aligned} g^{\alpha\beta} \phi_{,3} \Gamma_{\alpha\beta}^3 &\stackrel{0}{=} \phi_1 \left\{ \frac{2}{\delta} b_{\alpha\beta} \left( a^{\alpha\beta} + \frac{3\delta^2}{4} H b^{\alpha\beta} \right) + \frac{\delta}{2} b_{\alpha\gamma} b_\beta^\gamma b^{\alpha\beta} \right\} \\ &\quad \phi_2 \left\{ -2 b_{\alpha\gamma} b_\beta^\gamma \left( a^{\alpha\beta} + \frac{3\delta^2}{4} H b^{\alpha\beta} \right) + 4 b_{\alpha\beta} b^{\alpha\beta} - \frac{3\delta^2}{4} H b^{\alpha\beta} b_{\alpha\gamma} b_\beta^\gamma \right\} + \mathcal{O}\left((\delta\kappa)^2\right) \end{aligned} \quad (99)$$

$$= \frac{4H}{\delta} \phi_1 + 4(2H^2 - K) \phi_2 + \mathcal{O}\left((\delta\kappa)^2\right), \quad (100)$$

where the terms highlighted in orange can again be neglected based on Eqs. (65) and (66).

Using Eqs. (91), (92), (98), and (100) in Eq. (52), the Laplacian of the potential is expressed as

$$\begin{aligned} \Delta\phi &\stackrel{0}{=} \phi_{0,\alpha\beta} a^{\alpha\beta} + \frac{\delta}{2} b^{\alpha\beta} \phi_{1,\alpha\beta} + \frac{3\delta^2}{16} b^{\alpha\gamma} b_\gamma^\beta \phi_{2,\alpha\beta} + \frac{16}{\delta^2} \phi_2 - \\ &\quad \phi_{0,\gamma} \left\{ \left( {}^0\Gamma_{\alpha\beta}^\gamma - \frac{\delta^2}{8} b_{\alpha;\beta}^\mu b_\mu^\gamma \right) a^{\alpha\beta} - \frac{\delta^2}{4} b_{\alpha;\beta}^\gamma b^{\alpha\beta} \right\} - \\ &\quad \phi_{1,\gamma} \left\{ -\frac{\delta}{4} \left( b_{\alpha;\beta}^\gamma + \frac{3\delta^2}{8} H b_{\alpha;\beta}^\mu b_\mu^\gamma \right) a^{\alpha\beta} + \frac{\delta}{2} b^{\alpha\beta} \left( {}^0\Gamma_{\alpha\beta}^\gamma - \frac{3\delta^2}{16} b_{\alpha;\beta}^\mu b_\mu^\gamma \right) \right\} - \\ &\quad \phi_{2,\gamma} \left\{ -\frac{\delta^2}{16} b_{\alpha;\beta}^\mu b_\mu^\gamma a^{\alpha\beta} - \frac{\delta^2}{8} b^{\alpha\beta} b_{\alpha;\beta}^\gamma + \frac{3\delta^2}{8} H {}^0\Gamma_{\alpha\beta}^\gamma b^{\alpha\beta} \right\} \\ &\quad - \frac{4H}{\delta} \phi_1 - 4(2H^2 - K) \phi_2 + \mathcal{O}\left((\delta\kappa)^2\right) \end{aligned} \quad (101)$$

$$= \Delta^s \phi_0 - \frac{4}{\delta} H \phi_1 + \frac{16}{\delta^2} \phi_2 + \mathcal{O}\left((\delta\kappa)^2\right), \quad (102)$$

where the surface Laplacian is defined as  $\Delta^s \phi_0 = (\phi_{0,\alpha})_{;\beta} a^{\alpha\beta}$ , with the colon indicating the surface covariant derivative of a vector. The term highlighted in green is small based on Eqs. (60) and (61) and the terms highlighted in blue are negligible based on dimensional arguments. Namely, we assume there exists a characteristic in-plane length scale  $\ell$  over which the curvature and potential vary, satisfying

$$(\delta/\ell)^2 \ll 1. \quad (103)$$

Using Eqs. (59) and (103) and noting that Eq. (101) is invariant, non-dimensionalization allows us to neglect all terms highlighted in blue in Eq. (101). Also note that Eq. (102) is truncated at first

polynomial order which is equivalent to taking the inner product of the Laplacian with the zeroth order Chebyshev polynomial. Therefore, we can write the zeroth order contribution of Eq. (38) as

$$\varepsilon_M \Delta_s \phi_0(\zeta^\alpha) - 4C_M \phi_1(\zeta^\alpha) H + \frac{16}{\delta} C_M \phi_2(\zeta^\alpha) = 0, \quad (104)$$

where  $C_M = \varepsilon_M / \delta$  is the membrane capacitance per unit area.

Equation (104) has three unknowns, the coefficients  $\phi_0$ ,  $\phi_1$ , and  $\phi_2$ . As discussed in Sec. 4 of the main text, the jump conditions in Eqs. (37) and (39) are used to find expressions for  $\phi_1$  and  $\phi_2$ . To this end, we substitute the potential expansion, Eq. (88), into Eqs. (37) and (39), yielding

$$-\frac{2\varepsilon_M}{\delta} (\phi_1(\zeta^\alpha) + 4\phi_2(\zeta^\alpha)) = -\sigma^+ + \mathbf{n} \cdot \mathbf{e}_{B+}|_{\mathcal{S}^+}, \quad (105)$$

$$-\frac{2\varepsilon_M}{\delta} (\phi_1(\zeta^\alpha) - 4\phi_2(\zeta^\alpha)) = \sigma^- + \mathbf{n} \cdot \mathbf{e}_{B-}|_{\mathcal{S}^-}, \quad (106)$$

where  $\mathbf{e}_{B\pm}|_{\mathcal{S}^\pm}$  is the bulk electric field at the top and bottom bounding surfaces  $\mathcal{S}^\pm$ . Solving Eqs. (105) and (106) for  $\phi_1$  and  $\phi_2$  yields

$$\phi_1(\zeta^\alpha) = -\frac{1}{2C_M} \left( \mathbf{n} \cdot \langle \varepsilon_B \mathbf{e} \rangle^M - \frac{1}{2} (\sigma^+ - \sigma^-) \right), \quad (107)$$

$$\phi_2(\zeta^\alpha) = -\frac{1}{16C_M} \left( \mathbf{n} \cdot \llbracket \varepsilon_B \mathbf{e} \rrbracket^M - (\sigma^+ + \sigma^-) \right), \quad (108)$$

where  $\langle \varepsilon_B \mathbf{e} \rangle^M = \frac{1}{2} (\varepsilon_{B+} \mathbf{e}_{B+}|_{\mathcal{S}^+} + \varepsilon_{B-} \mathbf{e}_{B-}|_{\mathcal{S}^-})$  and  $\llbracket \varepsilon_B \mathbf{e} \rrbracket^M = \varepsilon_{B+} \mathbf{e}_{B+}|_{\mathcal{S}^+} - \varepsilon_{B-} \mathbf{e}_{B-}|_{\mathcal{S}^-}$  denote averages and jumps across the membrane, respectively. Equations (104), (107), and (108) are independent of the parametric direction  $\zeta^3$  and therefore, constitute the  $(2+\delta)$ -dimensional theory.

Finally, we derive effective boundary conditions corresponding to the three-dimensional boundary conditions in Eqs. (42) and (43). Expressing the expansion of the prescribed potential in terms of Chebyshev polynomials as

$$\bar{\phi}_M = \sum_{i=0}^{\infty} \bar{\phi}_{Mi} P_i(\theta), \quad (109)$$

and taking the inner product of Eq. (42) with the zeroth order Chebyshev polynomial yields

$$\phi_0 = \bar{\phi}_{M0}, \quad \forall \mathbf{x} \in \mathcal{S}_{||D}. \quad (110)$$

For the Neumann boundary condition in Eq. (43), we first note that the assumption of Kirchhoff-Love kinematics implies that the outward pointing normal (see Fig. 1) can be written as

$$\boldsymbol{\nu} = \nu^\alpha \mathbf{a}_\alpha, \quad (111)$$

where  $\nu_\alpha$  is independent of  $\zeta^3$ . Therefore, we find

$$\boldsymbol{\nu} \cdot \text{grad}(\phi) = (\phi_{,i} \mathbf{g}^i) \cdot (\nu^\alpha \mathbf{a}_\alpha) \quad (112)$$

$$= \nu^\alpha (\phi_{0,\beta} P_0(\theta) + \phi_{1,\beta} P_1(\theta) + \phi_{2,\beta} P_2(\theta)) \times \\ \left( \left( \delta_\alpha^\beta + \frac{\delta^2}{4} H b_\alpha^\beta \right) P_0(\theta) + \frac{\delta}{2} b_\alpha^\beta P_1(\theta) + \frac{\delta^2}{4} H b_\alpha^\beta P_2(\theta) \right) + \mathcal{O}((\delta\kappa)^2) \quad (113)$$

$$\stackrel{0}{=} \nu^\alpha \left( \phi_{0,\beta} \left( \delta_\alpha^\beta + \frac{\delta^2}{4} H b_\alpha^\beta \right) + \frac{\delta}{4} \phi_{1,\beta} b_\alpha^\beta + \frac{\delta^2}{16} \phi_{2,\beta} b_\gamma^\beta b_\alpha^\gamma + \mathcal{O}((\delta\kappa)^2) \right) , \quad (114)$$

where the term highlighted in orange can be neglected using Eqs. (65) and (66). Expanding the prescribed electric field as  $\bar{e} = \sum_{i=0}^{\infty} \bar{e}_i P_i(\theta)$  and taking the inner product of Eq. (114) with the zeroth order Chebyshev polynomial, Eq. (43) reduces to

$$-\nu^\alpha \left( \phi_{0,\alpha} + \frac{\delta}{4} \phi_{1,\beta} b_\alpha^\beta + \frac{\delta^2}{16} \phi_{2,\beta} b_\gamma^\beta b_\alpha^\gamma \right) = \bar{e}_0 , \quad (115)$$

where the equality only holds to order  $\mathcal{O}((\delta\kappa)^2)$ . When applying Eq. (115), we assume that  $\phi_1$  and  $\phi_2$  are determined by Eqs. (107) and (108), respectively. Alternatively, they could be determined by using the inner product of Eq. (43) with the first and second order Chebyshev polynomial.

### 3 Derivation of Analytical Solutions

In the following, the analytical solutions to the exact and  $(2+\delta)$ -dimensional theories used in Sec. 5.1 of the main text are derived. For the flat geometry, the  $(2+\delta)$ -dimensional theory is exact but for the cylinder and sphere, it deviates from the exact theory. Due to the curvature of the cylinder and sphere, the potential in the interior of the membrane does not just vary linearly and is thus not captured exactly by the  $(2+\delta)$ -dimensional theory. However, the error in the  $(2+\delta)$ -dimensional theory decreases quadratically with increasing radius of the geometry.

#### 3.1 Flat Geometry

Consider the flat geometry described in Sec. 5.1.1 of the main text. The governing equations for the three-dimensional theory are

$$\frac{d^2 \check{\phi}_{B^-}}{dx^2} = 0 , \quad \forall x \in (-\delta/2 - L^-, -\delta/2) , \quad (116)$$

$$\frac{d^2 \check{\phi}_M}{dx^2} = 0 , \quad \forall x \in (-\delta/2, \delta/2) , \quad (117)$$

$$\frac{d^2 \check{\phi}_{B^+}}{dx^2} = 0 , \quad \forall x \in (\delta/2, \delta/2 + L^+) , \quad (118)$$

together with the boundary conditions

$$-\frac{d\check{\phi}_{B^-}}{dx} = \bar{e} , \quad x = -\delta/2 - L^- , \quad (119)$$

$$\check{\phi}_{B^+} = 0 , \quad x = \delta/2 + L^+ , \quad (120)$$

and interface conditions

$$\check{\phi}_{B^-} = \check{\phi}_M , \quad x = -\delta/2 , \quad (121)$$

$$-\left( \varepsilon_M \frac{d\check{\phi}_M}{dx} - \varepsilon_B \frac{d\check{\phi}_{B^-}}{dx} \right) = \sigma^- , \quad x = -\delta/2 , \quad (122)$$

$$\check{\phi}_M = \check{\phi}_{B^+} , \quad x = \delta/2 , \quad (123)$$

$$-\left(\varepsilon_B \frac{d\check{\phi}_{B^+}}{dx} - \varepsilon_M \frac{d\check{\phi}_M}{dx}\right) = \sigma^+ , \quad x = \delta/2 . \quad (124)$$

Defining

$$\chi = \frac{\varepsilon_M}{\varepsilon_B} , \quad (125)$$

we can construct the piecewise solution for the exact theory as

$$\check{\phi}_{B^-} = -\bar{e}x + \bar{e} \left( \frac{\delta}{2} \left( \frac{2}{\chi} - 1 \right) + L^+ \right) + \frac{L^+}{\varepsilon_B} (\sigma^+ + \sigma^-) + \frac{\delta\sigma^-}{\varepsilon_M} , \quad (126)$$

$$\check{\phi}_M = -\left( \frac{\bar{e}}{\chi} + \frac{\sigma^-}{\varepsilon_M} \right) x + \bar{e} \left( \frac{\delta}{2\chi} + L^+ \right) + \frac{L^+}{\varepsilon_B} (\sigma^+ + \sigma^-) + \frac{\delta\sigma^-}{2\varepsilon_M} , \quad (127)$$

$$\check{\phi}_{B^+} = \left( -\bar{e} - \frac{1}{\varepsilon_B} (\sigma^+ + \sigma^-) \right) (x - (L^+ + \delta/2)) . \quad (128)$$

The governing equations of the  $(2 + \delta)$ -dimensional theory, Eqs. (104) and Gauss' law in the bulk domains, simplify to

$$\frac{d^2\phi_{B^-}}{dx^2} = 0 , \quad \forall x \in (-\delta/2 - L^-, -\delta/2) , \quad (129)$$

$$\phi_2 = 0 , \quad x = 0 , \quad (130)$$

$$\frac{d^2\phi_{B^+}}{dx^2} = 0 , \quad \forall x \in (\delta/2, \delta/2 + L^+) . \quad (131)$$

while the equations for  $\phi_1$  and  $\phi_2$ , Eqs. (107) and (108), read

$$-2C_M\phi_1 = -\frac{\varepsilon_B}{2} \left( \left. \frac{d\phi_{B^+}}{dx} \right|_{\frac{\delta}{2}} + \left. \frac{d\phi_{B^-}}{dx} \right|_{-\frac{\delta}{2}} \right) - \frac{1}{2} (\sigma^+ - \sigma^-) , \quad (132)$$

$$-16C_M\phi_2 = -\varepsilon_B \left( \left. \frac{d\phi_{B^+}}{dx} \right|_{\frac{\delta}{2}} - \left. \frac{d\phi_{B^-}}{dx} \right|_{-\frac{\delta}{2}} \right) - (\sigma^+ + \sigma^-) , \quad (133)$$

which enforce, by construction, the jump conditions in Eqs. (122) and (124), leaving us with the conditions for potential continuity on  $\mathcal{S}^\pm$ :

$$\phi_{B^-} = \phi_M , \quad x = -\delta/2 , \quad (134)$$

$$\phi_M = \phi_{B^+} , \quad x = \delta/2 . \quad (135)$$

The boundary conditions for the  $(2 + \delta)$ -dimensional theory remain as in the three-dimensional theory and are thus given by Eqs. (119) and (120).

The solutions in the bulk domains coincide with Eqs. (116) and (128), respectively, and are thus omitted here. In the membrane, the solution is defined by the three coefficients

$$\phi_0 = \bar{e} \left( \frac{\delta}{2\chi} + L^+ \right) + \frac{L^+}{\varepsilon_B} (\sigma^+ + \sigma^-) + \frac{\sigma^-}{2C_M} , \quad (136)$$

$$\phi_1 = -\frac{\delta}{2} \left( \frac{\bar{e}}{\chi} + \frac{\sigma^-}{\varepsilon_M} \right) , \quad (137)$$

$$\phi_2 = 0 , \quad (138)$$

and the expansion of the potential

$$\phi = \phi_0 P_0(\theta) + \phi_1 P_1(\theta) + \phi_2 P_2(\theta) . \quad (139)$$

The dimensionless coordinate  $\theta$  can be expressed as

$$\theta = \frac{2x}{\delta} , \quad (140)$$

and, by recalling the definition of the first three Chebyshev polynomials

$$P_0 = 1 , \quad (141)$$

$$P_1 = \theta , \quad (142)$$

$$P_2 = 2\theta^2 - 1 , \quad (143)$$

the expression for the potential in Eq. (139) yields the same result as the three-dimensional theory, Eq. (127).

### 3.2 Cylinders

Consider the cylindrical geometry described in Sec. 5.1.2 of the main text. With  $R_0^\pm = R_0 \pm \delta/2$ , the governing equations for the three-dimensional theory in cylindrical coordinates are

$$\frac{d}{dr} r \frac{d\check{\phi}_{B^-}}{dr} = 0 , \quad \forall r \in (R_A, R_0^-) , \quad (144)$$

$$\frac{d}{dr} r \frac{d\check{\phi}_M}{dr} = 0 , \quad \forall r \in (R_0^-, R_0^+) , \quad (145)$$

$$\frac{d}{dr} r \frac{d\check{\phi}_{B^-}}{dr} = 0 , \quad \forall r \in (R_0^+, R_E) , \quad (146)$$

together with the interface conditions

$$\check{\phi}_{B^-} = \check{\phi}_M , \quad r = R_0^- , \quad (147)$$

$$-\left( \varepsilon_M \frac{d\check{\phi}_M}{dr} - \varepsilon_B \frac{d\check{\phi}_{B^-}}{dr} \right) = \sigma^- , \quad r = R_0^- , \quad (148)$$

$$\check{\phi}_M = \check{\phi}_{B^+} , \quad r = R_0^+ , \quad (149)$$

$$-\left( \varepsilon_B \frac{d\check{\phi}_{B^+}}{dr} - \varepsilon_M \frac{d\check{\phi}_M}{dr} \right) = \sigma^+ , \quad r = R_0^+ . \quad (150)$$

Additionally, the potential is fixed to be zero at  $R_E > R_0^+$  and the electric field is imposed at  $0 < R_A < R_0^-$ :

$$-\frac{d\check{\phi}_{B^-}}{dr} = \bar{e} , \quad r = R_A , \quad (151)$$

$$\check{\phi}_{B+} = 0, \quad r = R_E. \quad (152)$$

The general form of the solution is

$$\check{\phi}_{B-} = -\bar{e}R_A \ln r + \check{B}^-, \quad (153)$$

$$\check{\phi}_M = \check{C} \ln r + \check{D}, \quad (154)$$

$$\check{\phi}_{B+} = \check{A}^+ \ln \frac{r}{R_E}, \quad (155)$$

with the remaining coefficients, determined using Eqs. (147)–(150),

$$\begin{aligned} \check{B}^- = & \left( \frac{\bar{e}R_A}{\chi} + \frac{R_0^- \sigma^-}{\varepsilon_M} \right) \ln \frac{R_0^+}{R_0^-} + \bar{e}R_A \ln R_0^- \\ & - \ln \frac{R_0^+}{R_E} \bar{e}R_A - \frac{1}{\varepsilon_B} \ln \frac{R_0^+}{R_E} (R_0^+ \sigma^+ + R_0^- \sigma^-), \end{aligned} \quad (156)$$

$$\check{A}^+ = -\bar{e}R_A - \frac{1}{\varepsilon_B} (R_0^- \sigma^- + R_0^+ \sigma^+), \quad (157)$$

$$\check{C} = -\frac{\bar{e}R_A}{\chi} - \frac{R_0^- \sigma^-}{\varepsilon_M}, \quad (158)$$

$$\check{D} = \left( \frac{\bar{e}}{\chi} R_A + \frac{R_0^- \sigma^-}{\varepsilon_M} \right) \ln R_0^+ - \left( \bar{e}R_A + \frac{1}{\varepsilon_B} (R_0^+ \sigma^+ + R_0^- \sigma^-) \right) \ln \frac{R_0^+}{R_E}. \quad (159)$$

For the dimensionally-reduced theory, the governing equations are

$$\frac{d}{dr} r \frac{d\phi_{B-}}{dr} = 0, \quad \forall r \in (R_A, R_0^-), \quad (160)$$

$$\frac{2C_M}{R_0} \phi_1 + \frac{16}{\delta} C_M \phi_2 = 0, \quad r = R_0, \quad (161)$$

$$\frac{d}{dr} r \frac{d\phi_{B-}}{dr} = 0, \quad \forall r \in (R_0^+, R_E), \quad (162)$$

where we used  $H = -1/(2R_0)$ . Similar to the flat geometry, the coefficients  $\phi_1$  and  $\phi_2$  are given by the equations

$$2C_M \phi_1 = \frac{\varepsilon_B}{2} \left( \left. \frac{d\phi_{B+}}{dr} \right|_{R_0+\frac{\delta}{2}} + \left. \frac{d\phi_{B-}}{dr} \right|_{R_0-\frac{\delta}{2}} \right) + \frac{1}{2} (\sigma^+ - \sigma^-), \quad (163)$$

$$16C_M \phi_2 = \varepsilon_B \left( \left. \frac{d\phi_{B+}}{dr} \right|_{R_0+\frac{\delta}{2}} - \left. \frac{d\phi_{B-}}{dr} \right|_{R_0-\frac{\delta}{2}} \right) + (\sigma^+ + \sigma^-). \quad (164)$$

As before, the jump conditions are satisfied by construction such that we only have to ensure continuity of the potential:

$$\phi_{B-} = \phi_M, \quad r = R_0^-, \quad (165)$$

$$\phi_M = \phi_{B+}, \quad r = R_0^+. \quad (166)$$

The boundary conditions remain as in the exact theory and are thus given by Eqs. (151) and (152).

The general form of the solutions to Eqs. (160)–(162) is

$$\phi_{B-} = -\bar{e}R_A \ln r + B^- , \quad (167)$$

$$\phi_M = \phi_0 P_0(\theta) + \phi_1 P_1(\theta) + \phi_2 P_2(\theta) , \quad (168)$$

$$\phi_{B+} = A^+ \ln \frac{r}{R_E} , \quad (169)$$

with the coefficients, determined using Eqs. (163)–(166),

$$\begin{aligned} \phi_0 = & \frac{\bar{e}R_A \delta}{16\chi R_0^- R_0^+} (8R_0 - \delta) + \frac{\delta}{16\varepsilon_M R_0^+} (\sigma^- (8R_0 - \delta)) \\ & - \left( \bar{e}R_A + \frac{1}{\varepsilon_B} (R_0^+ \sigma^+ + R_0^- \sigma^-) \right) \ln \left( \frac{R_0^+}{R_E} \right) , \end{aligned} \quad (170)$$

$$\phi_1 = -\frac{R_0 \delta (2\bar{e}\varepsilon_B R_A + 2R_0^- \sigma^-)}{4\varepsilon_M R_0^- R_0^+} , \quad (171)$$

$$\phi_2 = \frac{\bar{e}R_A \delta^2}{16\chi R_0^- R_0^+} + \frac{\delta \sigma^-}{16C_M R_0^+} , \quad (172)$$

$$A^+ = -\bar{e}R_A - \frac{1}{\varepsilon_B} (R_0^- \sigma^- + R_0^+ \sigma^+) , \quad (173)$$

$$\begin{aligned} B^- = & \frac{\bar{e}R_A R_0 \delta}{\chi R_0^- R_0^+} + \frac{R_0 \sigma^-}{C_M R_0^+} + \bar{e}R_A \ln R_0^- \\ & - \ln \frac{R_0^+}{R_E} \bar{e}R_A - \frac{1}{\varepsilon_B} \ln \frac{R_0^+}{R_E} (R_0^+ \sigma^+ + R_0^- \sigma^-) . \end{aligned} \quad (174)$$

Comparison of the bulk solutions of the three-dimensional and  $(2+\delta)$ -dimensional theories shows exact agreement for  $r \geq R_0^+$ , i.e.  $\phi_{B+} = \check{\phi}_{B+}$ . However, for  $r < R_0^+$ , the  $(2+\delta)$ -dimensional theory is not exact. Defining the non-dimensional curvature as

$$\mu = \frac{\delta}{2R_0} , \quad (175)$$

the error between the exact and  $(2+\delta)$ -dimensional theories scales quadratically with  $\mu$  for  $r < R_0^-$ , i.e.  $\phi_{B-} - \check{\phi}_{B-} = \mathcal{O}(\mu^2)$ , consistent with the assumption in Eq. (59). For comparison within the membrane, the exact potential is expressed as

$$\check{\phi}_M = -\left( \frac{\bar{e}R_A}{\chi} + \frac{R_0^- \sigma^-}{\varepsilon_M} \right) \ln \left( \frac{r}{R_0^+} \right) - \left( \bar{e}R_A + \frac{1}{\varepsilon_B} (R_0^+ \sigma^+ + R_0^- \sigma^-) \right) \ln \frac{R_0^+}{R_E} . \quad (176)$$

Evaluating the inner product of Eq. (176) proves difficult such that we instead expand the first logarithmic term:

$$\ln \left( \frac{r}{R_0^+} \right) = \ln \left( \frac{R_0 + \delta/2\theta}{R_0 + \delta/2} \right) \quad (177)$$

$$= \sum_{n=1}^{\infty} (-1)^{(n-1)} \frac{1}{n} \left( \frac{\mu(\theta-1)}{1+\mu} \right)^n . \quad (178)$$

Given that  $\frac{\mu}{1+\mu} < 1$ , the constant, linear, and quadratic contribution are, respectively,

$$-\sum_{n=1}^{\infty} \frac{1}{n} \left( \frac{\mu}{1+\mu} \right)^n = -\ln(1+\mu) = -\mu + \mathcal{O}(\mu^2) , \quad (179)$$

$$\sum_{n=1}^{\infty} \left( \frac{\mu}{1+\mu} \right)^n \theta = \mu \theta , \quad (180)$$

$$-\sum_{n=1}^{\infty} \frac{(n-1)}{2} \left( \frac{\mu}{1+\mu} \right)^n \theta^2 = -\frac{\mu^2}{2} \theta^2 . \quad (181)$$

Thus, the constant part of Eq. (176) can be written as

$$\frac{\bar{e}R_A\delta}{2R_0\chi} + \frac{R_0^-\delta\sigma^-}{2\varepsilon_M R_0} - \left( \bar{e}R_A + \frac{1}{\varepsilon_B} (R_0^+\sigma^+ + R_0^-\sigma^-) \right) \ln \frac{R_0^+}{R_E} . \quad (182)$$

while the linear term takes the form

$$-\frac{\bar{e}R_A\delta}{2R_0\chi} - \frac{R_0^-\delta\sigma^-}{2\varepsilon_M R_0} , \quad (183)$$

and the quadratic term becomes

$$\frac{\bar{e}R_A\delta^2}{8\chi R_0^2} + \frac{R_0^-\delta^2\sigma^-}{8\varepsilon_B R_0^2} . \quad (184)$$

By rewriting the  $(2+\delta)$ -dimensional solution in standard polynomial form, i.e.

$$\phi_M = \phi_0 - \phi_2 + \phi_1\theta + 2\phi_2\theta^2 , \quad (185)$$

the constant contribution of the  $(2+\delta)$ -dimensional solution evaluates to

$$\begin{aligned} \phi_0 - \phi_2 = & \frac{\bar{e}R_A\delta R_0}{2\chi R_0^- R_0^+} \left( 1 - \frac{\mu}{2} \right) + \frac{R_0\sigma^-}{2C_M R_0^+} \left( 1 - \frac{\mu}{2} \right) \\ & - \left( \bar{e}R_A + \frac{1}{\varepsilon_B} (R_0^+\sigma^+ + R_0^-\sigma^-) \right) \ln \left( \frac{R_0^+}{R_E} \right) . \end{aligned} \quad (186)$$

Comparing Eq. (186) to Eq. (182), Eq. (171) to Eq. (183), and Eq. (172) to Eq. (184) shows that the error between the exact and  $(2+\delta)$ -dimensional theories scales as  $\mathcal{O}(\mu^2)$ , again consistent with Eq. (59).

### 3.3 Spheres

Consider the spherical geometry described in Sec. 5.1.3 of the main text. The governing equations for the three-dimensional theory in spherical coordinates are

$$\frac{d}{dr} r^2 \frac{d\check{\phi}^-}{dr} = 0 , \quad \forall r \in (R_A, R_0^-) , \quad (187)$$

$$\frac{d}{dr} r^2 \frac{d\check{\phi}_M}{dr} = 0 , \quad \forall r \in (R_0^-, R_0^+) , \quad (188)$$

$$\frac{d}{dr} r^2 \frac{d\check{\phi}^-}{dr} = 0, \quad \forall r \in (R_0^+, R_E). \quad (189)$$

The interface and boundary conditions remain as in the cylindrical case and are thus given by Eqs. (147)–(152). Upon applying the boundary conditions, Eqs. (151) and (152), the general form of the solution becomes

$$\check{\phi}^- = \check{e} \frac{R_A^2}{r} + \check{B}^-, \quad (190)$$

$$\check{\phi}_M = -\frac{\check{C}}{r} + \check{D}, \quad (191)$$

$$\check{\phi}^+ = \frac{\check{A}^+}{R_E} \left( \frac{R_E}{r} - 1 \right), \quad (192)$$

with the remaining constants determined using the interface conditions, Eqs. (147)–(150):

$$\check{A}^+ = \frac{1}{\varepsilon_B} \left( \sigma^+ (R_0^+)^2 + \sigma^- (R_0^-)^2 \right) + e R_A^2, \quad (193)$$

$$\begin{aligned} \check{B}^- = \frac{\delta}{R_0^+ R_0^-} \left( \frac{e R_A^2}{\chi} + \frac{\sigma}{\varepsilon_B} (R_0^-)^2 \right) - \frac{e R_A^2}{R_0^- R_0^+ R_E} (\delta R_E + R_0^+ R_0^-) \\ - \frac{1}{\varepsilon_B R_0^+ R_E} (R_0^+ - R_E) \left( \sigma^+ (R_0^+)^2 + \sigma^- (R_0^-)^2 \right), \end{aligned} \quad (194)$$

$$\check{C} = -\frac{e R_A^2}{\chi} - \frac{\sigma^-}{\varepsilon_M} (R_0^-)^2, \quad (195)$$

$$\begin{aligned} \check{D} = -\frac{1}{R_0^+ \chi} \left( e R_A^2 + \frac{\sigma^-}{\varepsilon_B} (R_0^-)^2 \right) - \frac{e R_A^2 (R_0^+ - R_E)}{R_0^+ R_E} \\ - \frac{(R_0^+ - R_E)}{\varepsilon_B R_0^+ R_E} \left( \sigma^+ (R_0^+)^2 + \sigma^- (R_0^-)^2 \right). \end{aligned} \quad (196)$$

For the dimensionally-reduced theory, the governing equations are

$$\frac{d}{dr} r^2 \frac{d\phi^-}{dr} = 0, \quad \forall r \in (R_A, R_0^-), \quad (197)$$

$$C_M \frac{4}{R_0} \phi_1 + \frac{16}{\delta} C_M \phi_2 = 0, \quad r = R_0, \quad (198)$$

$$\frac{d}{dr} r^2 \frac{d\phi^-}{dr} = 0, \quad \forall r \in (R_0^+, R_E), \quad (199)$$

where we have used  $H = -1/R_0$ . The interface conditions, the governing equations for  $\phi_1$  and  $\phi_2$ , as well as the boundary conditions remain the same as in the cylindrical case and are thus given by Eqs. (163)–(166). After applying the boundary conditions, the general form of the solution reads

$$\phi^- = e \frac{R_A^2}{r} + B^-, \quad (200)$$

$$\phi_M = \phi_0 P_0(\theta) + \phi_1 P_1(\theta) + \phi_2 P_2(\theta), \quad (201)$$

$$\phi^+ = \frac{A^+}{R_E} \left( \frac{R_E}{r} - 1 \right), \quad (202)$$

with the remaining coefficients determined using Eqs. (163)–(166):

$$\begin{aligned} \phi_0 = & -\frac{\delta^2}{8\chi(R_0 + \delta)} \left( e \left( \frac{R_A}{R_0^-} \right)^2 + \frac{\sigma^-}{\varepsilon_B} \right) - \frac{R_0(R_0^+ - R_E) e R_A^2}{R_0^+(R_0 + \delta) R_E} - \\ & \frac{R_0 R_0^+(R_0^+ - R_E)(\sigma^+ + \sigma^-)}{\varepsilon_B(R_0 + \delta) R_E} + \frac{\delta R_0 e R_A^2}{2\chi(R_0 + \delta)(R_0^-)^2} + \frac{R_0 \sigma^-}{2C_M(R_0 + \delta)} \\ & - \frac{\delta(R_0^+ - R_E) R_0^+}{(R_0 + \delta) R_E} \left( -e \frac{R_A^2}{(R_0^-)^2} + \frac{(\sigma^+ - \sigma^-)}{\varepsilon_B} \right), \quad (203) \end{aligned}$$

$$\phi_1 = -\frac{\delta R_0 e R_A^2}{2\chi(R_0 + \delta)(R_0^-)^2} - \frac{R_0 \sigma^-}{2C_M(R_0 + \delta)}, \quad (204)$$

$$\phi_2 = \frac{\delta^2 e R_A^2}{8\chi(R_0 + \delta)(R_0^-)^2} + \frac{\delta \sigma^-}{8C_M(R_0 + \delta)}, \quad (205)$$

$$A^+ = e R_A^2 \frac{(R_0 - \delta)(R_0^+)^2}{(R_0 + \delta)(R_0^-)^2} + \frac{(R_0^+)^2 \sigma^+}{\varepsilon_B} + \frac{(R_0^+)^2 (R_0 - \delta) \sigma^-}{\varepsilon_B(R_0 + \delta)}, \quad (206)$$

$$\begin{aligned} B^- = & \frac{\delta R_0}{(R_0 + \delta)} \left( \frac{e R_A^2}{(R_0^-)^2 \chi} + \frac{\sigma^-}{\varepsilon_M} \right) - \frac{e R_A^2 R_0 - \delta}{R_E R_0 + \delta} \left( \frac{R_0^+}{R_0^-} \right)^2 \\ & - e R_A^2 \frac{\delta R_0}{(R_0 + \delta)(R_0^-)^2} - \frac{R_0^+}{\varepsilon_B R_E} (R_0^+ - R_E) \left( \sigma^+ + \sigma^- \frac{R_0 - \delta}{R_0 + \delta} \right). \quad (207) \end{aligned}$$

The functional forms of the solution of the exact and  $(2 + \delta)$ -dimensional theories coincide in the bulk domains such that it is sufficient to compare the coefficients  $\check{A}^+$  and  $A^+$  as well as  $\check{B}^-$  and  $B^-$ . Expanding the respective expressions around  $\mu = 0$  shows that  $A^+$  and  $B^-$  are accurate up to order  $\mathcal{O}(\mu^2)$ , with  $\mu$  defined in Eq. (175).

To compare the solutions within the membrane, we expand the exact solution in Eq. (191) around  $\mu = 0$ :

$$\check{\phi}_M = -\frac{\check{C}}{r} + \check{D} \quad (208)$$

$$= -\frac{\check{C}}{R_0(1 + \mu\theta)} + \check{D} \quad (209)$$

$$= -\frac{\check{C}}{R_0} \sum_{k=0}^{\infty} (-1)^k \mu^k \theta^k + \check{D}. \quad (210)$$

The series converges for  $|\mu| < |\theta|^{-1}$ , which is satisfied since  $\theta \in (-1, 1)$  and  $|\mu| < 1$ . Therefore, we identify the constant part of  $\check{\phi}_M$  as  $-\frac{\check{C}}{R_0} + \check{D}$  and comparison to  $\phi_0 - \phi_2$  shows that the constant contribution of the  $(2 + \delta)$ -dimensional theory is accurate up to order  $\mathcal{O}(\mu^2)$ . Similarly, we can compare  $\frac{\check{C}}{R_0} \mu$  to  $\phi_1$  and  $-\frac{\check{C}}{R_0} \mu^2$  to  $\frac{1}{2}\phi_2$ , also revealing accuracy to order  $\mathcal{O}(\mu^2)$  as expected by the assumptions of the  $(2 + \delta)$ -dimensional theory.

## References

- [1] Kovetz, A. *Electromagnetic theory*, vol. 975 (Oxford University Press Oxford, 2000).
- [2] Casey, J. On the derivation of jump conditions in continuum mechanics. *The international journal of structural changes in solids* **3**, 61–84 (2011).
- [3] Fong, K. D., Bergstrom, H. K., McCloskey, B. D. & Mandadapu, K. K. Transport phenomena in electrolyte solutions: Nonequilibrium thermodynamics and statistical mechanics. *AIChE journal* **66**, e17091 (2020).
- [4] Melcher, J. R. *Continuum electromechanics*, vol. 2 (MIT press Cambridge, 1981).
- [5] Jackson, J. D. *Classical electrodynamics* (1999).
- [6] Itskov, M. *et al. Tensor algebra and tensor analysis for engineers* (Springer, 2007).
- [7] Sauer, R. A. & Duong, T. X. On the theoretical foundations of thin solid and liquid shells. *Mathematics and mechanics of solids* **22**, 343–371 (2017).
